# Supplementary material for: GReTA - a novel Global and Recursive Tracking Algorithm in three dimensions
Source: arXiv:1305.1495 ancillary file (2015-04-17)
Supplement: Supplementary file 1 [file AncillaryFile1_Appendices.pdf]

## APPENDIX A

### DATA-TAKING PROCEDURES

Two distinct but similar experimental setups are used to acquire the video sequences of flocking starlings (*Sturnus Vulgaris*) and swarming midges (*Chironomidae* and *Ceratopogonidae*) in the field. Despite the scale difference between the two setups, they both rely on the same system of industrial high-speed cameras IDT-M5 ([www.idtpiv.com](http://www.idtpiv.com), monochromatic CMOS sensor  $2288 \times 1728$  pixels @ 170 Hz). Each camera-head is connected via a double Camera-Link cable to a processing unit, which hosts a frame-grabber and a RAID hard-drive array for data storage. For midge experiments, 50 mm  $f/2.8$  lenses are used together with infrared filters to reduce the infrared component of the direct sunlight hitting the background. For bird video acquisitions, 28 mm  $f/2.0$  and 16 mm  $f/2.0$  lenses are used. The two setups also share the same geometry, which is schematically shown in Fig. 7: two cameras are separated by a baseline distance  $D_{12}$ , which is proportional to the working distance  $Z_W$  (i.e. the distance of the flock or swarm from the cameras). We also use a third camera, placed at the shorter distance  $D_{23}$  from the second one, which allow us to use the trifocal stereometric geometry – as described in Appendix C. In the case of birds, the mutual positions and orientations of the cameras are accurately measured on the field, as described by Cavagna *et al.* [1]. In this case, typically  $D_{12} = 25.0$  m,  $D_{23} = 2.5$  m, and  $Z_W \in [90; 200]$  m. In the case of midges, the mutual positions and orientations are instead retrieved from a set of images of a known linear target [2]. For the midge setup, typically  $D_{12} = 3.0$  m,  $D_{23} = 0.25$  m, and  $Z_W \in [4; 10]$  m. For both experiments, intrinsic camera parameters (i.e. optical distortions and aberrations) are also retrieved with a calibration routine which makes use of a set of images of a known planar target.

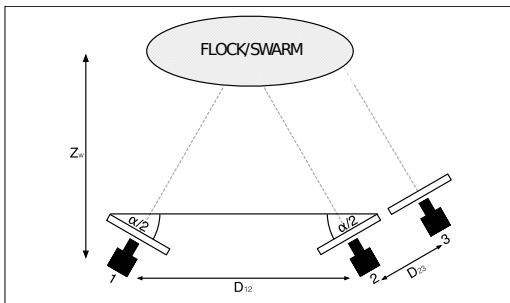

Fig. 7. Schematic drawing of the geometry of the experimental setups used to acquire flocking starlings data and swarming midges data in the field.

## APPENDIX B

### IMAGE SEGMENTATION

We developed an image segmentation routine to detect the objects in the experimental images, specifically

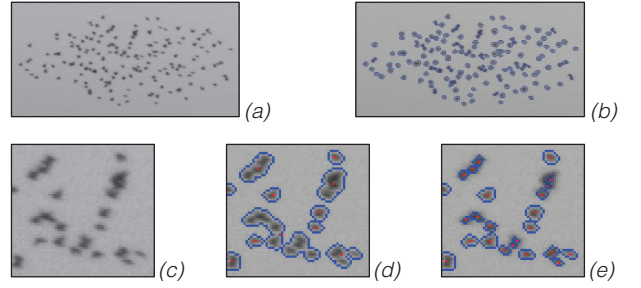

Fig. 8. The individual steps of the image segmentation routine applied to photographs of flocking birds.

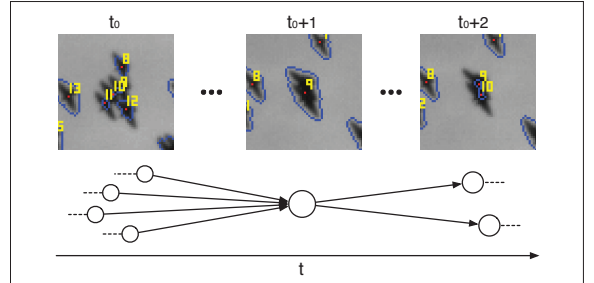

Fig. 9. Example of partly occluding objects in an image, which the watershed technique of our segmentation routine failed to split. The path-branching approach allows linking the four distinct objects detected at frame  $t_0$  to the single object which represents the same four objects at the following frame  $t_0 + 1$ , and this one with the two distinct objects detected at the subsequent frame  $t_0 + 2$ .

tailored to our data: irregularly shaped birds, dark on a bright background; bright circular images of midges, back-scattering direct sunlight at sunset, in front of a dark unsteady background. A sample photograph of flocking birds is shown in Fig. 8: in panel (a), a crop of an original photograph of a flock is shown; in panel (c), a crop of a few dozens of birds of the same original photograph is shown.

The implemented routine computes the background of each individual image on the images within a time-window centered around the current frame. The background is subtracted, and a Gaussian denoising algorithm is used. An intensity threshold is applied to the images to extract binary pixel maps. A two-pass labeling algorithm [3] finds interconnected regions on the binary maps, identifying them as target objects (marked in blue in Fig. 8(d)). Using a weighted average [4], the centroid coordinates of each target object are extracted (marked as red dots in Fig. 8(d)). A watershed technique permits splitting clusters of adjacent or partly occluded objects, as shown in Fig. 8(e) (flock crop) and Fig. 8(b) (full flock). Cases of unsolved occlusions are shown in Fig. 9. A detailed description of the entire segmentation routine is reported in Cavagna *et al.* [1].

## APPENDIX C

### STEREOSCOPIC AND TEMPORAL LINKING

The assignment of stereoscopic links and the one of temporal links are completely independent from each other, and are performed in the 2D space of each camera. Thanks to this, our method is very robust to the presence of wrong links, because a wrong stereoscopic link does not influence the assignment of temporal links, and *vice versa*.

The procedures we use to assign stereoscopic and temporal links share the same global optimization strategy used to match 2D paths. The choice of the specific cost functions being optimized depends on the number of cameras used to acquire the scene, and on the individual and collective motion kinematics of the objects, for stereoscopic and temporal links, respectively.

#### C.1 Stereoscopic linking

We match the individual 2D objects across the images acquired by three cameras optimizing globally in space (*i.e.* over all objects in the three images for each time instant) the function:

$$\min_{x_{ijk}^S} \sum_{ijk} f(d_{ijk}^S) x_{ijk}^S, \quad (1)$$

$$\text{with the constraints: } \begin{aligned} \forall i \quad \sum_{jk} x_{ijk}^S &\geq 1, \\ \forall j \quad \sum_{ki} x_{ijk}^S &\geq 1, \\ \forall k \quad \sum_{ij} x_{ijk}^S &\geq 1, \end{aligned} \quad (2)$$

where  $i, j, k$  are the object indices in the images of the first, second, and third camera, respectively;  $d_{ijk}^S$  is the three-dimensional tensor of the stereometric distances between the  $i$ -th,  $j$ -th, and  $k$ -th objects;  $x_{ijk}^S$  is a three-dimensional boolean tensor of the variables of the optimization problem (true if the  $i$ -th,  $j$ -th, and  $k$ -th objects are matched, false if not);  $f(d_{ijk}^S)$  is a cost function used to weight the stereometric distances. The cost function we choose is  $f(d_{ijk}^S) = (d_{ijk}^S)^2$ . There are several possible definitions of the stereometric distance; we prefer to use the trifocal distance (see [5]) to the sum of the epipolar distances, because the trifocal geometry presents less degeneracies. The meaning of this distance is the following: given the objects  $i, j, k$  on the images, with perfect calibration of the setup and in absence of noise, it would be zero if the triplet  $i, j, k$  is a correct match (*i.e.* it corresponds to a real 3D-object in space), and larger than zero otherwise. In practice, when the optical density is large, stereometric distances of false and correct matches can be of the same order, making the assignment of stereoscopic links non-trivial. This is why an optimization procedure is required.

Note that a crucial element of our global optimization scheme is encoded in (2). Standard assignment algorithms assume a strict equality as a constraint,

which means that each object  $i$  in an image corresponds to only one object  $j$  and to one object  $k$  in the other two images (*i.e.* only one  $x_{ijk}^S$  can be different from zero). On the contrary, we use a non-strict equality requirement, and we therefore allow the possibility to assign multiple links per object, which is an essential feature of our tracking method.

#### C.2 Temporal linking

We follow exactly the same approach to assign temporal links. First, we choose a kinematic prediction strategy with which we predict the position at time  $(t + 1)$  of the  $i$ -th object at time  $t$ . We then link the individual objects in time across the frames of the photo-sequences optimizing globally in space (*i.e.* over all objects for each time instant) the function:

$$\min_{x_{ij}^T} \sum_{ij} f(d_{ij}^T) x_{ij}^T, \quad (3)$$

$$\text{with the constraints: } \begin{aligned} \forall i \quad \sum_j x_{ij}^T &\geq 1, \\ \forall j \quad \sum_i x_{ij}^T &\geq 1, \end{aligned} \quad (4)$$

where  $i$  and  $j$  are the indices of the objects at time  $t$  and  $(t + 1)$ , respectively;  $d_{ij}^T$  is the tensor of the two-dimensional distances between the predicted position of the  $i$ -th object and the  $j$ -th candidate;  $x_{ij}^T$  is a boolean tensor of the variables of the optimization problem (true if the  $i$ -th and  $j$ -th objects are linked, false if not);  $f(d_{ij}^T)$  is a cost function used to weight the distances. We choose  $f(d_{ij}^T) = (d_{ij}^T)^2$  again as the cost function. As before, the possibility to assign multiple links per object is expressed in (4) by the non-strict equality requirement. Different prediction strategies are used for birds and midges. We found that a roto-scale-translation predicts well the highly-polarized flight kinematics of birds flying within a flock, and we estimate its parameters at every time instant using the Kabsch algorithm [6]. A two-times constant velocity prediction approach, or a three-times constant acceleration prediction approach [7], are used in case of swarming midges, whose flight directions are highly uncorrelated. The difficulty of the temporal linking problem can be quantified in terms of the ratio  $\xi = \langle v \rangle \Delta t / \Delta r$ , where  $\langle v \rangle$  is the average speed of the objects in the 2D image-space,  $\Delta t$  is the temporal delay between consecutive acquired images, and  $\Delta r$  the average inter-object 2D distance. Typically, our  $\xi$  ranges between 0.02 and 0.3.

During the evaluation of the possible candidate objects for stereoscopic and temporal linking, we set a threshold on the distances  $d^S$  and  $d^T$  over which we discard physically impossible matches. Both optimization problems are solved using a linear programming algorithm, for which we use the C++ APIs of *IBM ILOG CPLEX Optimization Studio v12.2* [8].

## APPENDIX D

### THEOREM 1

We formalize here the existence and uniqueness of the solution of the tracking problem under suitable hypotheses.

*Theorem 1: Under the hypotheses:*

- 1) the sets of temporal links and stereoscopic links contain all and only the correct links;
- 2) the cost function has zero noise, i.e.  $c = 0$  if two objects are stereoscopically linked,  $c = 1$  otherwise;
- 3) each object is not occluded by other objects at least in one image of one camera during the entire temporal sequence;
- 4) an object  $A$  which is occluded by object  $B_1$  at time  $t_1$ , and by object  $B_2$  at time  $t_2 > t_1$  in the images of the same camera, is not occluded by any other object for at least one instant of time  $t \in [t_1, t_2]$ ;
- 5) two objects  $A_1$  and  $A_2$  which occlude each other in the images of one camera in the time interval  $[t_1, t_2]$ , do not occlude each other in the images of at least one other camera in the time interval  $[t_1 - 1, t_2 + 1]$ ;
- 6) each tracked object is detected in the images of each camera during the entire temporal sequence.

The correct solution of the tracking problem is the only cover set which minimizes the cost defined by Eq. 2 with the constraint Eq. 3.

This implies the equivalence  $\Gamma_{opt} \equiv G$ .

*Proof of Theorem 1:* For the sake of simplicity, the proof is given for a system of two cameras and it can be easily generalized to systems with more than two cameras. In order to prove Theorem 1, the following lemma is necessary.

*Lemma 1: Under the hypotheses of Theorem 1, the set  $G$  of the correct trajectories is the only solution of the problem with cost  $c(G) = 0$ .*

*Proof of Lemma 1:* Each track  $g \in G$  is a sequence of linked 2D objects. Hypothesis 1 assures that all and only the temporal links exist, so that all the correct 2D paths in each camera space can be created. Hypothesis 2 implies that their cost is zero. Therefore the cost of the set  $G$ , which is the sum of the costs of all correct trajectories, is equal to zero – which is a minimum for the cost function.

Let us prove that  $G$  is the only solution with cost equal to zero. Assume the existence of another set of trajectories  $\Gamma \neq G$ , for which  $c(\Gamma) = 0$ . Since  $\Gamma \neq G$ , there exists a trajectory  $\gamma \in \Gamma$  which does not belong to  $G$  ( $\gamma \notin G$ ) and which cost is zero. The set  $G$  covers all the segmented objects. This implies that each 2D object in  $\gamma$  belongs to at least one trajectory in  $G$ . Formally, there exist  $g_1, \dots, g_m, h_1, \dots, h_n \in G$  such that:

$$\gamma_1^i = \begin{cases} (g_1)_1^i & i \in [1, \dots, T^1] \\ \vdots \\ (g_m)_1^i & i \in (T^{m-1}, \dots, T] \end{cases} \quad (5)$$

and

$$\gamma_2^i = \begin{cases} (h_1)_2^i & i \in [1, \dots, S^1] \\ \vdots \\ (h_n)_2^i & i \in (S^{n-1}, \dots, T] \end{cases} \quad (6)$$

with  $1 \leq T^1 < \dots < T^m = T$  and  $1 \leq S^1 < \dots < S^n = T$ .

For the sake of simplicity, we consider here only the cases for which  $m, n = 1, 2$ , and a generalization for  $m, n > 2$  can be obtained with the same arguments. Let us analyze separately the cases  $m = n = 1$  and  $m = 2$ , the latter being exactly equivalent to the case  $n = 2$ . Let us indicate with  $\gamma_i^h$  the element (i.e., a 2D object) of the trajectory  $\gamma$  at time  $i$  in camera  $h$ .

**m=n=1.** The trajectory  $\gamma$  coincides with  $g_A$  in the first camera, and with  $h_B$  in the second camera, where  $g_A$  and  $h_B$  are two distinct trajectories in  $G$  representing the two real objects  $A$  and  $B$ , respectively. Formally:

$$\forall i \in [1, \dots, T], \quad \gamma_1^i = (g_A)_1^i \text{ and } \gamma_2^i = (g_B)_2^i. \quad (7)$$

The trajectories  $g_A$  and  $g_B$  are in  $G$ , their cost is therefore equal to 0, and  $c_\gamma = 0$  by definition. Hypotheses 1 and 2 assure that there exist all the stereoscopic links  $((g_A)_1^i, (g_A)_2^i)$ ,  $((h_B)_1^i, (h_B)_2^i)$  and  $(\gamma_1^i, \gamma_2^i) = ((g_A)_1^i, (h_B)_2^i)$ . This implies the existence of three objects:  $A$ , represented by  $g_A$ ;  $B$ , represented by  $h_B$ ; and a third object, represented by  $\gamma$ , which at each instant of time is occluded in the first camera view by object  $A$ , and in the second camera view by object  $B$ . This is forbidden by Hypothesis 4.

**m=2.** In this case, the 2D objects of  $\gamma$  in the first camera view belong to two different trajectories,  $g_A$  and  $g_B$  in  $G$ . The 2D path of  $\gamma$  in the same camera view is completely occluded by  $g_A$  during the temporal interval  $[1, T^1]$ , and it is completely occluded by  $g_B$  the following interval  $[T^1 + 1, T]$ . Formally, for the first camera view:

$$\gamma_1^i = \begin{cases} (g_A)_1^i & i \in [1, \dots, T^1] \\ (g_B)_1^i & i \in (T^1, \dots, T] \end{cases} \quad (8)$$

with  $(g_A)_1^{T^1} \neq (g_B)_1^{T^1}$ , or  $(g_A)_1^{T^1+1} \neq (g_B)_1^{T^1+1}$ .

Let us first consider the case for which:

$$(g_A)_1^{T^1} \neq (g_B)_1^{T^1} \text{ and } (g_A)_1^{T^1+1} \neq (g_B)_1^{T^1+1}. \quad (9)$$

The two objects  $A$  and  $B$ , corresponding to  $g_A$  and  $g_B$ , respectively, are distinct at time  $T^1$  as well as at time  $T^1 + 1$ . The presence of the temporal link  $(\gamma_1^{T^1}, \gamma_1^{T^1+1})$ , together with Hypothesis 1, implies the existence of a real object occluded by  $A$  at frame  $T^1$  and by  $B$  at frame  $T^1 + 1$ . This is forbidden by Hypothesis 5.

Assume that

$$(g_A)_1^{T^1} = (g_B)_1^{T^1} \text{ and } (g_A)_1^{T^1+1} \neq (g_B)_1^{T^1+1}. \quad (10)$$

Since  $m = 2$ , there exists a time  $T^0 < T^1$  such that  $(g_A)_1^{T^0-1} \neq (g_B)_1^{T^0-1}$ . The objects  $A$  and  $B$ , represented by  $g_A$  and  $g_B$ , occlude each other in the first

camera view within the entire interval  $[T^0, \dots, T^1]$ . In this case, the path  $g_{AGB}$  exists, but it cannot represent a real object: in fact, the object should be occluded at time  $T^0 - 1$  with  $A$  and at time  $T^1 + 1$  with  $B$ , therefore being occluded by  $A$  and  $B$  during the entire interval  $[T^0, T^1]$ . This is forbidden by Hypothesis 4. We can conclude that, in the first camera view,  $\gamma$  can only be a representation of an hybrid object with  $c(\gamma) = 0$ .

Making use of Hypothesis 1 once more,  $\forall i \in [1, \dots, T]$  there exist the stereoscopic links  $((g_A)_1^i, (g_A)_2^i)$ ,  $((g_B)_1^i, (g_B)_2^i)$  and  $(\gamma_1^i, \gamma_2^i)$ , with:

$$(\gamma_1^i, \gamma_2^i) = \begin{cases} ((g_A)_1^i, (g_A)_2^i) & i \in [1, \dots, T^0] \\ ((g_B)_1^i, (g_B)_2^i) & i \in (T^1, \dots, T] \end{cases} \quad (11)$$

Such equation implies the existence of a temporal link connecting  $g_A$  and  $g_B$  in the second camera view for  $i \in [T^0, T^1]$ . As in the previous case,  $\gamma$  in the second camera view can only represent an hybrid object. In order to preserve the stereometric coherency, the objects  $A$  and  $B$  must occlude each other during at least one time instant in the interval  $[T^0, T^1]$  – in contrast with Hypothesis 4.

The same arguments can be used to prove that the existence of  $\gamma \in \Gamma$ ,  $\gamma \notin G$  and  $c(\gamma) = 0$  is forbidden by Hypotheses 4, 5, and 6 of Theorem 1 in the case of  $(g_A)_1^{T^1} \neq (g_B)_1^{T^1}$  and  $(g_A)_1^{T^1+1} = (g_B)_1^{T^1+1}$ . Hence,  $G$  is the only cover set with cost equal to zero.

*Proof of Theorem 1:* Lemma 1 assures that  $G$  is the only solution with cost equal to zero. This implies that it is the solution with minimum cost, and the solution found by the global optimization algorithm is the correct one,  $G$ .

*Proof of Corollary 1:* If Hypotheses 1-6 are satisfied within each recursive interval, the partial correct solution with cost equal to zero is found within each interval. Connecting together these partial solutions, one obtains the full correct trajectories, and the cost of the solution is zero.

## APPENDIX E NUMERICAL SIMULATION FOR SYNTHETIC DATASETS

Ground-truth trajectories are generated running a simple three-dimensional self-propelled particle model [9], described by the following system of equations:

$$\frac{d\vec{v}_i}{dt} = -\frac{k_1}{n_c} \sum_{j \in \pi_i} (\vec{v}_i - \vec{v}_j) - k_2 \frac{\vec{v}_i}{v_i} (v_i - v_0) + \frac{k_3}{n_c} \sum_{j \in \pi_i} \vec{f}_{ij} + \sqrt{\eta} \vec{v}_i, \quad (12)$$

$$\frac{d\vec{x}_i}{dt} = \vec{v}_i(t). \quad (13)$$

Here,  $\pi_i$  represents the interaction ensemble of bird  $i$  at time  $t$ , determined by a topological rule;  $n_c$  is the number of interacting neighbors of bird  $i$ ;  $v_i = |\vec{v}_i|$  is the modulus of the velocity  $\vec{v}_i$ , expressed by Eq. 13 as

the temporal derivative of the position vector  $\vec{x}_i$ . The attraction-repulsion force term  $\vec{f}_{ij}$  is defined as:

$$\vec{f}_{ij} = \frac{\vec{r}_{ij}}{r_{ij}} \begin{cases} \frac{1}{4} \frac{r_{ij} - r_e}{r_e} & \text{if } r_{ij} < 2r_e, \\ 1 & \text{otherwise.} \end{cases} \quad (14)$$

The last term of Eq. 12 is defined as the noise amplitude  $\sqrt{\eta}$  times the random vector  $\vec{v}_i$  with zero mean and unit variance:  $\langle \nu_i^m(t) \nu_j^n(t') \rangle = \delta_{i,j} \delta_{m,n} \delta_{t,t'}$ , with  $m, n = x, y, z$ . The model parameters  $k_1, k_2, k_3, \eta, v_0$ , and  $r_e$  are chosen to simulate a realistic behavior of flocking birds, with characteristic length and time scales comparable to the ones observed in field experimental data:  $k_1 = 4.0 \text{ s}^{-1}$ ;  $k_2 = 2.0 \text{ s}^{-1}$ ;  $k_3 = 2.0 \text{ ms}^{-2}$ ;  $\eta = 1.5 \text{ m}^2 \text{ s}^{-4}$ ;  $v_0 \in [7.0, 18.0] \text{ m/s}$ ;  $r_e \in [1.5, 2.5] \text{ m}$  (equilibrium distance). The simulation is discretized using a time-step equal to  $1/170 \text{ s}$ , corresponding to the highest frame-rate used to acquire the experimental datasets (see Appendix A). As initial conditions for the simulation, all particles are uniformly distributed in a sphere, and their initial velocities are aligned with the  $x$ -axis.

The 3D-positions along the generated trajectories are then projected on three simulated camera planes using a typical set of projection matrices retrieved from the calibrations of our experimental datasets. The used projection matrices roughly correspond to the geometry described in Appendix A and in Fig. 7 therein, with  $D_{12} = 25.0 \text{ m}$ ,  $D_{23} = 2.5 \text{ m}$ , and  $Z_W \simeq 130.0 \text{ m}$ .

In order to simulate the segmentation error, we add a random normally distributed noise with standard deviation  $\sigma$  to the projected 2D coordinates. To this aim we choose  $\sigma$  to mimic the noise typical of our experimental data. We also simulate optical occlusions for groups of  $n \geq 2$  simulated birds whose mutual 2D distances are shorter than a threshold radius, for which we use the typical image size of the birds in our experimental images (3 pixels). The coordinates of the birds which happen to be closer than the threshold radius are set equal to the coordinates of the center of mass of the group of occluding birds.

## REFERENCES

- [1] A. Cavagna, I. Giardina, A. Orlandi, G. Parisi, A. Procaccini, M. Viale, and V. Zdravkovic, The STARFLAG handbook on collective animal behaviour: Part I, empirical methods. *Animal Behaviour* **76**, 217–236 (2008).
- [2] A. Attanasi, A. Cavagna, L. Del Castello, I. Giardina, S. Melillo, L. Parisi, O. Pohl, B. Rossaro, E. Shen, E. Silvestri, and M. Viale, Collective behaviour without collective order in wild swarms of midges, *PLoS Computational Biology* **10**, 7, 1–15 (2014).
- [3] L.G. Shapiro and G.C. Stockman, *Computer Vision*, first ed. Upper Saddle River, N.J.: Prentice-Hall, 2001.
- [4] R. Parthasarathy, Rapid, accurate particle tracking by calculation of radial symmetry centers. *Nat. Methods* **9**, 724–726 (2012).
- [5] R. Hartley and A. Zisserman, *Multiple View Geometry in Computer Vision*, second ed. Cambridge, U.K.: Cambridge University Press, 2003.
- [6] W. Kabsch, A solution for the best rotation to relate two sets of vectors. *Acta Crystallographica* **32**, 922 (1976).

- [7] N.T. Ouellette, H. Xu, and E. Bodenschatz, A quantitative study of three-dimensional Lagrangian particle tracking algorithms. *Exp. Fluids* **40**, 301–313 (2006).
- [8] CPLEX Optimization Incorporated, *Using the CPLEX Callable Library*, Incline Village, Nevada, 1994.
- [9] W. Bialek, A. Cavagna, I. Giardina, T. Mora, O. Pohl, E. Silvestri, M. Viale, and A. Walczak, Social interactions dominate speed control in poising natural flocks near criticality. *Proceedings of the National Academy of Sciences* , **111**, 20, 7212–7217 (2014).
